# Supplementary material for: A behavioural transformer for effective collaboration between a robot and a non-stationary human
Source: arXiv:2307.13447 source file (2023-07-25)
Supplement: Supplementary file 1 [file appendix.tex]

\newpage
\quad % without \quad no new page would be insert!!!
\newpage

\subsection{Prediction of the latent state}
The prediction of future latent states $\hat{z}_{t+1}$ are explicit functions of past latent states $(z_t,z_{t-1},...)$, the current and past time-index features $((s,a_R )_t,[(s,a_R)]_{t-1},...)$ and exogenous (human) factors ($z_H$).

\subsection{Dataset}
10 humans. Play 20 games with each human. The human’s hit the ball back and forth between four locations. 

\subsection{Nomenclature}
\begin{itemize}
    \item Episode number: $i \in \{0, ...,I'\}$.
    \item Human number: $N \in \{0, ..., N'\}$.
    \item Timestep: $t \in \{0, ..., T\}$
    \item Number of humans: $I' = 10$
    \item Number of episodes per human $N' = 20$
    \item Time at episode $i$ for human $N$: $t_N^i$
    \item Local observability 
    \begin{equation}
    \begin{split}
    S = (x_{Ball}, y_{Ball}, v_{x,Ball}, \\ v_{y,Ball}, y_{paddle}, O_{paddle}, H_{number}
    \end{split}
    \end{equation}
    \item Action human $a_H = y_{Ball} | x_{Ball} = x_{min}$
    \item Human data $\tau = \{ (s, a, r, s'), ... , (s, a, r, s')$
    
\end{itemize}

\subsection{Nomenclature?}

\begin{tabular}{l l }
$\mathit{x_{Ball}}$ & x position ball \\ 
$\mathit{y_{Ball}}$ & y position ball \\  
$\mathit{v_{x, Ball}}$ & x velocity ball \\ 
$\mathit{v_{y, Ball}}$ & y velocity ball \\ 
$\mathit{O_{paddle}}$ & paddle orientation) \
 \end{tabular}

 \section{Dynamics of custom environment}
The (deterministic) physical dynamics for the simplest discrete case is described below. In the simplest case the ball follows the orientation of the paddle rather than realistic physical dynamics. Physical dynamics will be included in more complex versions of the game.

The custom platform allows empirical investigation of the impact of manipulating various factors on learning. The complexity of the environment will be increased systematically in several ways. For example, the time it takes the ball to travel from one end to the other can be adjusted parametrically (affecting the sparsity of the rewards). Obstacles can be added, and different reward values  given when hitting the ball to different regions. It is also possible to investigate both discrete and continuous state and action spaces.\\

\noindent The rules of the proposed experiments are summarised below:\\

\noindent \textbf{Common Goal:} Achieve the maximum score.\\
\textbf{Episode ends when:} (i) the robot misses (ii) 1 minute is up.\\
\textbf{Score:} +1 for every time the ball hits a paddle.\\

\noindent \textbf{State space $S$}: $S = \{P_1, P_2, O_1, O_2, X_B, Y_B, V_{x_B}, V_{y_B}\}$

\begin{itemize} %[label={}]
\item Paddle 1 position, $P_1 = [0, 100, 200]$
\item Paddle 2 position, $P_2 = [0, 100, 200]$
\item Paddle 1 orientation, $O_1 = [0, 100, 200]$
\item Paddle 2 orientation, $O_2 = [0, 100, 200]$
\item Ball x-position, $x_B = [0, 100, 200]$
\item Ball y-position, $y_B = [0, 100, 200]$
\item Ball x-velocity, $V_{x_B} = [0, 100, 200]$
\item Ball y-velocity, $V_{y_B} = [0, 100, 200]$
\end{itemize}

    \noindent \textbf{Action space $S$}: $A = \{a_{up}, a_{down}, a_{clockwise}, a_{anticlockwise}\}$

\begin{itemize} %[label={}]
\item $[1, 0, 0, 0] \implies$ up
\item $[0, 1, 0, 0] \implies$ down
\item $[0, 0, 1, 0] \implies$ rotate clockwise
\item $[0, 0, 0, 1] \implies$ rotate anticlockwise
\end{itemize}

\noindent \textbf{Reward $R$}
\begin{equation}
    R^a_{ss'} = +1\ \forall a\ \text{where for}\ s'\ \text{ball-position = paddle-position}.\end{equation}
\begin{equation}
R^a_{ss'} = -10\ \forall a\ \text{where for}\ s'\ \text{$x_B < x_{min}$ or $x_B > x_{max}$}.
\end{equation}

\noindent where $x_{min}$ and $x_{max}$ are the minimum and maximum bounds in the x-direction for the ball respectively.\\

\noindent \textbf{Discount factor}
$\gamma$ = 1 (no discounting) as a high negative reward is recieved at the termination of the episode.\\

\noindent \textbf{Dynamics $T$}
The (deterministic) physical dynamics for the simplest discrete case is described below. In the simplest case the ball follows the orientation of the paddle rather than realistic physical dynamics. Physical dynamics will be included in more complex versions of the game.

\begin{equation}
t_{t+1} = t_t + 1
\end{equation}
\begin{equation}
x_{t+1} = x_t + v_{x}t
\end{equation}
\begin{equation}
y_{t+1} = y_t + v_{y}t
\end{equation}
\begin{equation}
P_{1,t+1} = P_{1,t} + a_{P_{1,t}}
\end{equation}
\begin{equation}
P_{2,t+1} = P_{2,t} + a_{P_{2,t}}
\end{equation}
\begin{equation}
O_{1,t+1} = O_{1,t} + a_{O_{1,t}}
\end{equation}
\begin{equation}
V_{x,t+1} = V_{x,t},\ V_{y,t+1} = V_{y,t}\ \text{if no collision}
\end{equation}
\begin{equation}
V_{x,t+1} = -V_{x,t}\ \text{if collision}
\end{equation}
\begin{equation}
V_{y,t+1} = -V_{x,t} \cdot \sin{\alpha}\ \text{if collision, where $\alpha$ is the orientation of the paddle}
\end{equation}

\subsection{Details of the components of the human behaviour}

\subsection{Influence component}
\begin{equation}
P(z_{inf}) = 
\begin{cases}
    \text{0.4},& \text{if } a_{R,inf} = z_i\\
    {0.2},              & \text{otherwise}
\end{cases}
\end{equation}

\subsection{Low frequency hysteresis}

\begin{equation}
z_{low} \sim \rho_{low} (\Bar{z}^{i-1})
\end{equation}

\subsection{High frequency hysteresis}

\begin{equation}
z_{high} \sim \rho_{high} (z^i_{t-2}, z^i_{t-1})
\end{equation}

\subsection{Constant (time-invariant) component}

\begin{equation}
p(L) = 0.3, p(R) = 1 - p(L) = 0.7
\end{equation}

\begin{equation}
P(z_c | L) = 
\begin{cases}
    \text{Beta($\alpha = 5, \beta = 4$)},& \text{for } z_{c,i} = 0\\
    {\frac{1 - P(z_{c,3} | L)}{3}},              & \text{otherwise}
\end{cases}
\end{equation}

\begin{equation}
P(z_c | R) = 
\begin{cases}
    \text{Beta($\alpha = 5, \beta = 4$)},& \text{for } z_{c,i} = 3\\
    {\frac{1 - P(z_{c,3} | R)}{3}},              & \text{otherwise}
\end{cases}
\end{equation}
